# Supplementary material for: Diagnosing and Rectifying Vision Models using Language
Source: arXiv:2302.04269 source file (2023-02-08)
Supplement: Supplementary file 1 [file domino_fairface_id.pdf]

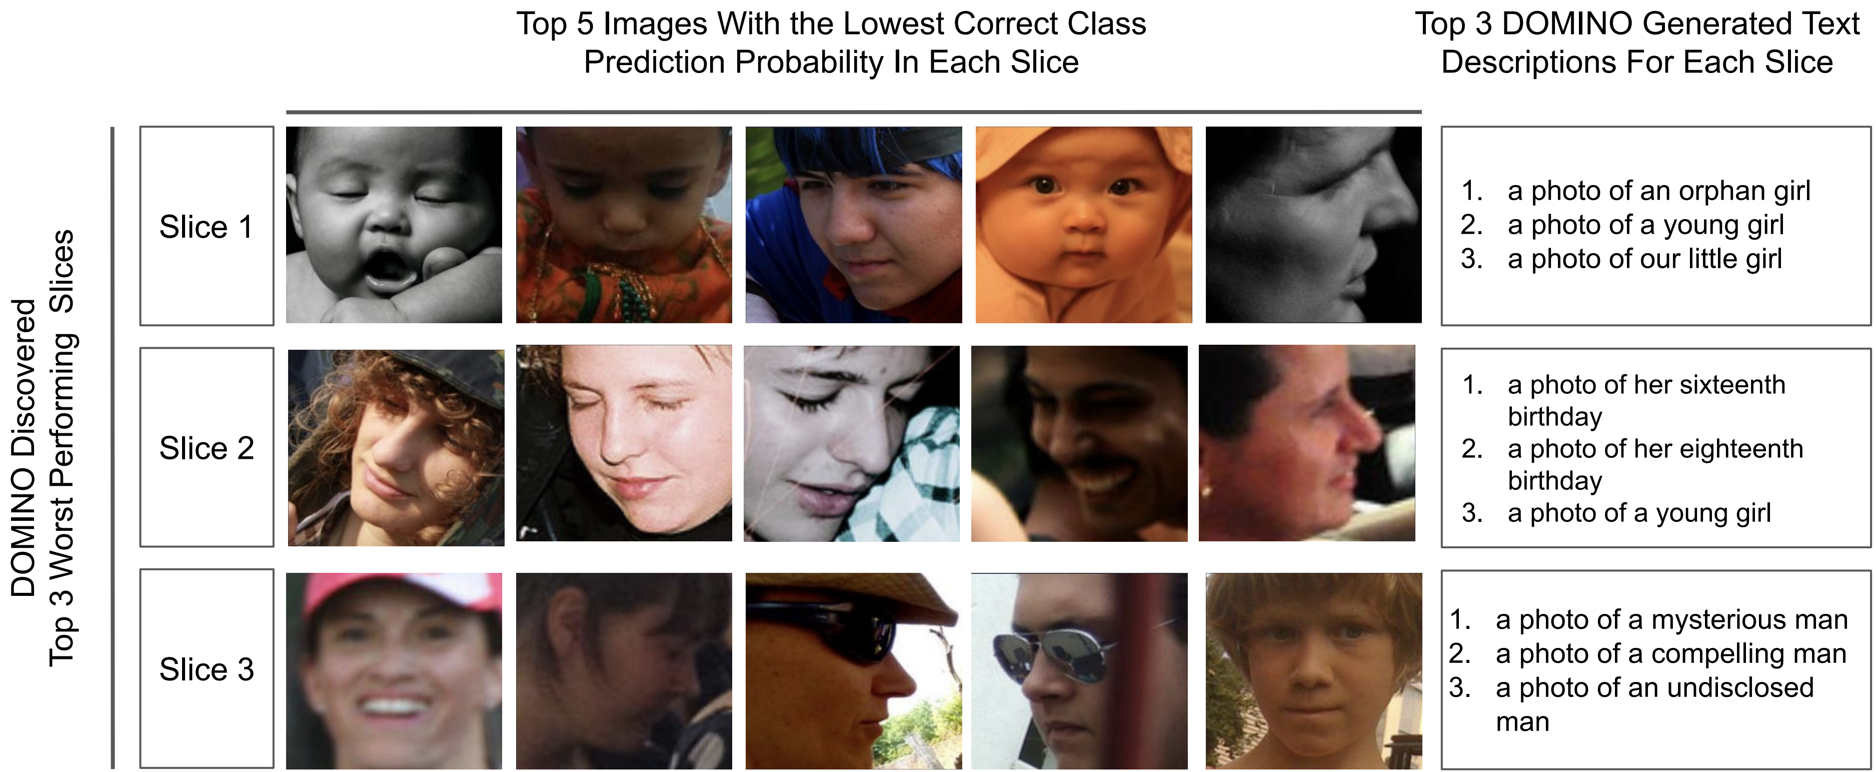

Top 5 Images With the Lowest Correct Class Prediction Probability In Each Slice
Top 3 DOMINO Generated Text Descriptions For Each Slice
DOMINO Discovered Top 3 Worst Performing Slices
Slice 1
1. a photo of an orphan girl
2. a photo of a young girl
3. a photo of our little girl
Slice 2
1. a photo of her sixteenth birthday
2. a photo of her eighteenth birthday
3. a photo of a young girl
Slice 3
1. a photo of a mysterious man
2. a photo of a compelling man
3. a photo of an undisclosed man

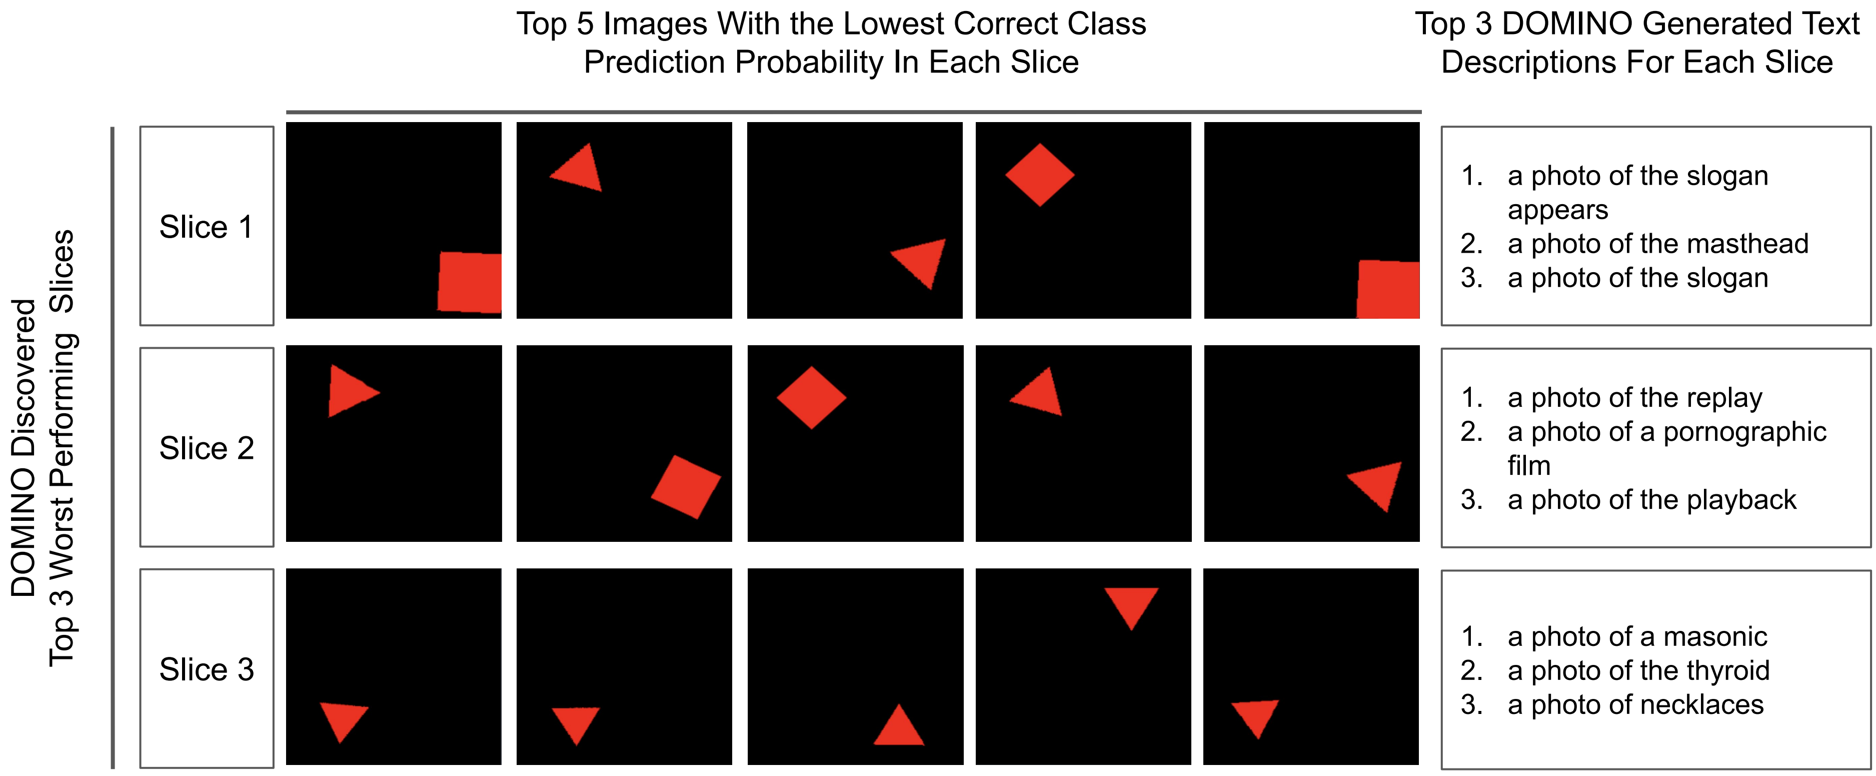
Top 5 Images With the Lowest Correct Class Prediction Probability In Each Slice
Top 3 DOMINO Generated Text Descriptions For Each Slice
DOMINO Discovered Top 3 Worst Performing Slices
Slice 1
1. a photo of the slogan appears
2. a photo of the masthead
3. a photo of the slogan
Slice 2
1. a photo of the replay
2. a photo of a pornographic film
3. a photo of the playback
Slice 3
1. a photo of a masonic
2. a photo of the thyroid
3. a photo of necklaces

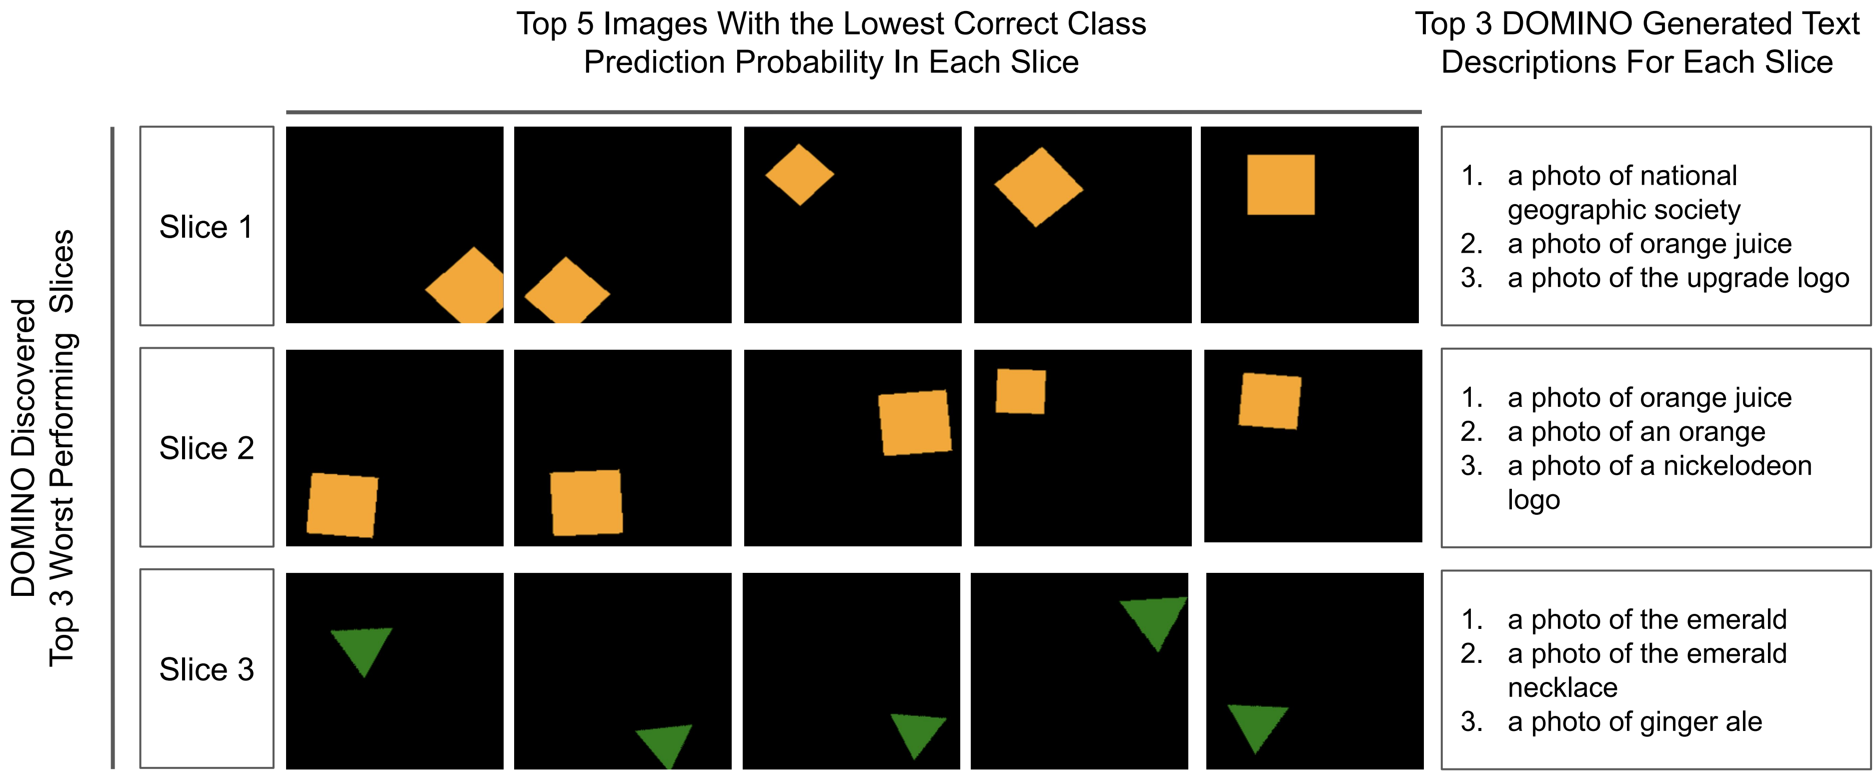
Top 5 Images With the Lowest Correct Class Prediction Probability In Each Slice
Top 3 DOMINO Generated Text Descriptions For Each Slice
DOMINO Discovered Top 3 Worst Performing Slices
Slice 1
1. a photo of national geographic society
2. a photo of orange juice
3. a photo of the upgrade logo
Slice 2
1. a photo of orange juice
2. a photo of an orange
3. a photo of a nickelodeon logo
Slice 3
1. a photo of the emerald
2. a photo of the emerald necklace
3. a photo of ginger ale
